# Supplementary material for: Controlled abstention neural networks for identifying skillful predictions for classification problems
Source: arXiv:2104.08281 ancillary file (2021-04-16)
Supplement: Supplementary file 1 [file Barnes_Barnes_2021_suppClass.pdf]

# Supporting Information for "Controlled abstention neural networks for identifying skillful predictions for classification problems"

Elizabeth A. Barnes[1] and Randal J. Barnes[2]

[1]Department of Atmospheric Science, Colorado State University, Fort Collins, CO, USA.

[2]Civil, Environmental, and Geo- Engineering, University of Minnesota, Minneapolis, MN, USA.

## Contents of this file

1. Text S1
2. Figures S1 to S3

## Text S1: Proof of Theorem for NotWrong Loss

### Notation

- There are $k$ classes, which we number $1, 2, \ldots, k$.
- We append a pseudo-class to allow for abstention, which we number $k+1$.
- Let $x$ denote a sample with true label $j$, where $1 \leqslant j \leqslant k$.
- Let $[a_1, a_2, \ldots, a_k, a_{k+1}]$ be the network output before the softmax.
- Let $[p_1, p_2, \ldots, p_k, p_{k+1}]$ be the output from the softmax.
- $\alpha$ is a non-negative weight.

In keeping with standard terminology, we will call $p_i$ the *likelihood* that sample $x$ belongs to class $i$ as predicted by the model.

### NotWrong Loss Function

The NotWrong loss function can be written as

$$\boxed{\mathcal{L}(x) = -\log(r+s) - \alpha \log(q)} \tag{1}$$

where

- $q = (1 - p_{k+1})$ is the likelihood of **not** abstaining,
- $r = p_j$ is the likelihood of being correct, and
- $s = p_{k+1}$ is the likelihood of abstaining.

Note that $q + s = 1$.

**Theorem Considered**

Thulasidasan et al. (2019) introduces the DAC loss function for abstention networks and Thulasidasan (2020, Chapter 3) explores the DAC loss function and presents the following theorem:

Theorem 1. For the (DAC) loss function $L$ given in Equation 3.1, if $j$ is the given class for sample $x$, then as long as $\alpha \geqslant 0$, $\frac{\partial L}{\partial a_j} \leqslant 0$ (where $a_j$ is the pre-activation into the softmax unit of class $j$).

Does this theorem also apply to the NotWrong loss function as well? We apply the chain rule and write

$$\frac{\partial \mathcal{L}}{\partial a_j} = \frac{\partial \mathcal{L}}{\partial q}\frac{\partial q}{\partial a_j} + \frac{\partial \mathcal{L}}{\partial r}\frac{\partial r}{\partial a_j} + \frac{\partial \mathcal{L}}{\partial s}\frac{\partial s}{\partial a_j} \tag{2}$$

The various pieces are

$$\frac{\partial \mathcal{L}}{\partial q} = -\frac{\alpha}{q} \tag{3}$$
$$\frac{\partial \mathcal{L}}{\partial r} = -\frac{1}{r+s} \tag{4}$$
$$\frac{\partial \mathcal{L}}{\partial s} = -\frac{1}{r+s} \tag{5}$$

and for $j \in \{1, 2, \ldots, k\}$

$$\frac{\partial q}{\partial a_j} = \frac{\partial(1-p_{k+1})}{\partial a_j} = p_j \cdot p_{k+1} = r \cdot s \tag{6}$$
$$\frac{\partial r}{\partial a_j} = \frac{\partial p_j}{\partial a_j} = p_j - p_j^2 = r - r^2 \tag{7}$$
$$\frac{\partial s}{\partial a_j} = \frac{\partial p_{k+1}}{\partial a_j} = -p_j \cdot p_{k+1} = -r \cdot s \tag{8}$$

Substituting (3) - (8) back into (2), and simplifying, we find

$$\frac{\partial \mathcal{L}}{\partial a_j} = \left(-\frac{\alpha}{q}\right)(r \cdot s) + \left(-\frac{1}{r+s}\right)(r - r^2) + \left(-\frac{1}{r+s}\right)(-r \cdot s) \tag{9}$$
$$= -\frac{\alpha r s}{q} - \frac{r - r^2}{r+s} + \frac{rs}{r+s} \tag{10}$$
$$= -r\left(\frac{\alpha s}{q} + \frac{q - r}{r+s}\right) \tag{11}$$
$$= -p_j\left(\frac{\alpha p_{k+1}}{1-p_{k+1}} + \frac{1 - p_j - p_{k+1}}{p_j + p_{k+1}}\right) \tag{12}$$

Since $p_i \geqslant 0$ for all $i$, and $\sum_{i=1}^{k+1} p_i = 1$

$$\leqslant 0 \tag{13}$$

Thus, Theorem 1 applies to the NotWrong loss function and states that during gradient descent, the learning on the true class of a given sample persists even when the network has abstained on the sample.

**The *softmax***

The following derivation with the *softmax* is used in the proof of Theorem 1 above. The *softmax* takes the network output a's and generates p's using

$$\boxed{p_i = \frac{e^{a_i}}{\sum_{n=1}^{k+1} e^{a_n}}} \tag{14}$$

for $i = 1, 2, \ldots, k+1$. Consequently, $p_i \geqslant 0$ for all $i$, and $\sum_{i=1}^{k+1} p_i = 1$.

The derivatives of the *softmax* outputs with respect to the *softmax* inputs for $i \neq j$ are

$$\frac{\partial p_i}{\partial a_j} = \frac{\partial}{\partial a_j}\left(\frac{e^{a_i}}{\sum_{n=1}^{k+1} e^{a_n}}\right) \tag{15}$$

$$= -\frac{e^{a_i} \cdot e^{a_j}}{\left(\sum_{n=1}^{k+1} e^{a_n}\right)^2} \tag{16}$$

$$= -\frac{e^{a_i}}{\sum_{n=1}^{k+1} e^{a_n}} \cdot \frac{e^{a_j}}{\sum_{n=1}^{k+1} e^{a_n}} \tag{17}$$

$$= -p_i \cdot p_j \tag{18}$$

For $i = j$, we have

$$\frac{\partial p_j}{\partial a_j} = \frac{\partial}{\partial a_j}\left(\frac{e^{a_j}}{\sum_{n=1}^{k+1} e^{a_n}}\right) \tag{19}$$

$$= \frac{e^{a_j}\left(\sum_{n=1}^{k+1} e^{a_n}\right) - e^{a_j}e^{a_j}}{\left(\sum_{n=1}^{k+1} e^{a_n}\right)^2} \tag{20}$$

$$= \frac{e^{a_j}}{\sum_{n=1}^{k+1} e^{a_n}} - \frac{e^{a_j}}{\sum_{n=1}^{k+1} e^{a_n}} \cdot \frac{e^{a_j}}{\sum_{n=1}^{k+1} e^{a_n}} \tag{21}$$

$$= p_j - p_j^2 \tag{22}$$

In summary,

$$\boxed{\frac{\partial p_i}{\partial a_j} = \begin{cases} -p_i \cdot p_j & i \neq j \\ p_j - p_j^2 & i = j \end{cases}} \tag{23}$$

## Supplemental Figures S1 to S3

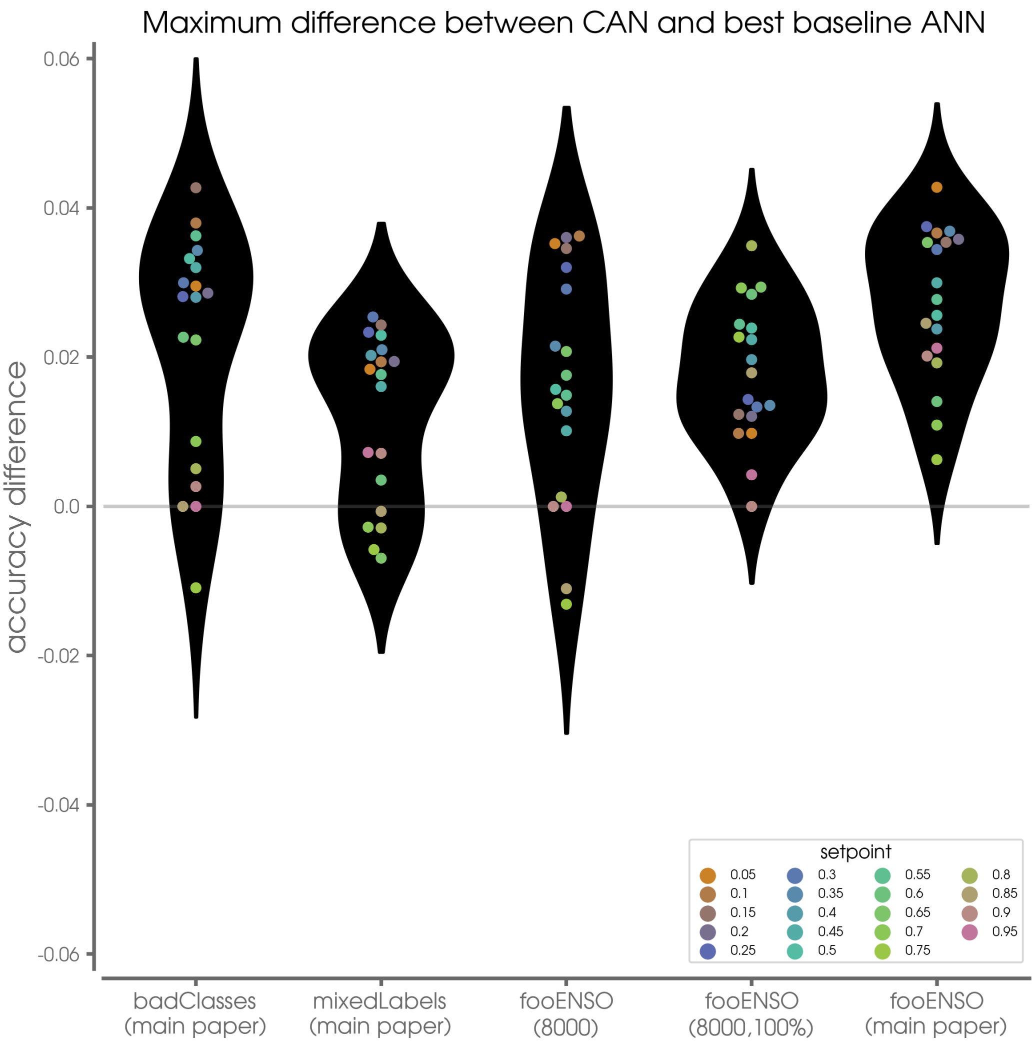


**Figure S1.** Maximum difference in testing accuracy between the CAN and the best baseline ANN for various abstention setpoints across five different experiments. Positive values imply higher accuracies of the CAN compared to the best baseline ANN. "fooENSO (8000)" denotes a similar experiment to the main paper's fooENSO experiment, except training over 8,000 samples only (with the simpler network architecture) and "fooENSO (8000,100%)" is the same except 100% of the non-El Niño samples are corrupted, rather than only 50%.

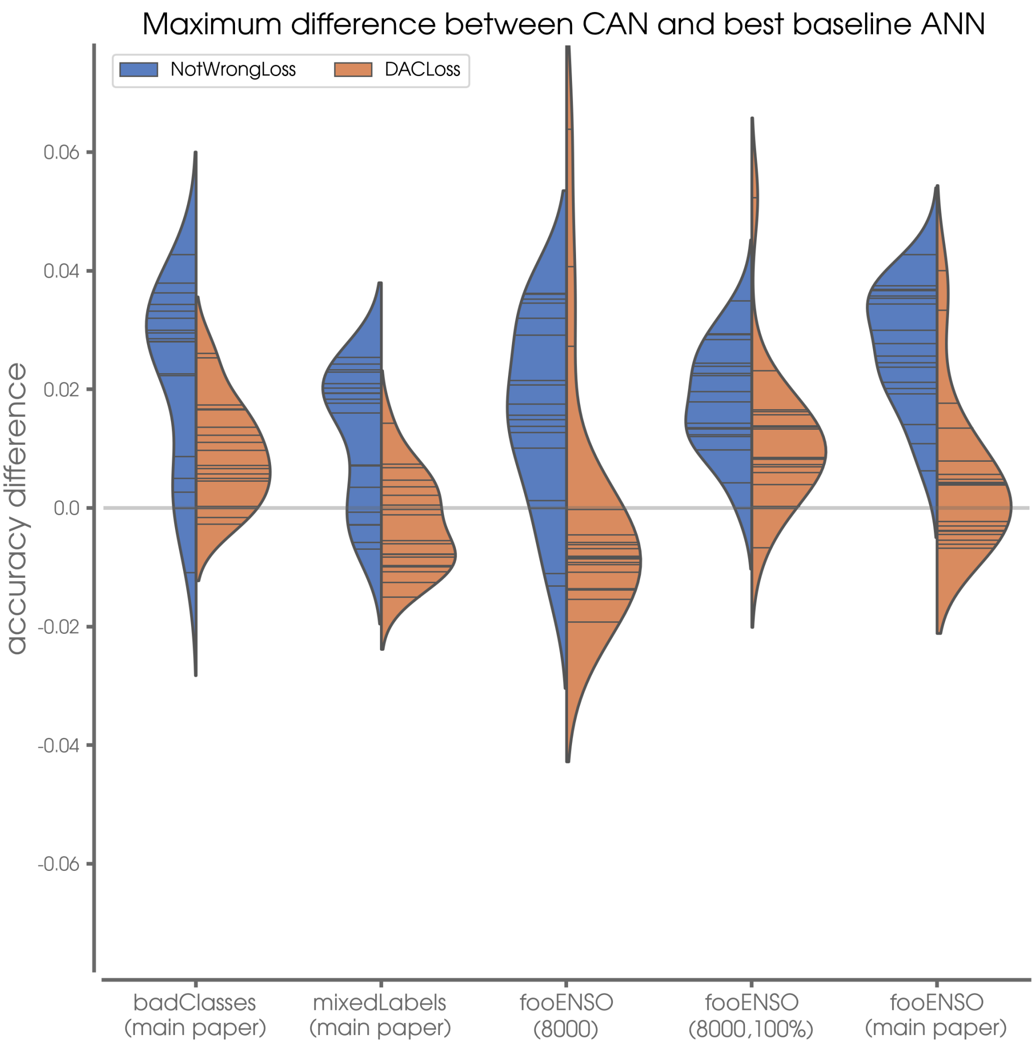


**Figure S2.** Maximum difference in testing accuracy between the CAN and the best baseline ANN for various abstention setpoints across five different experiments and two loss functions. Positive values imply higher accuracies of the CAN compared to the best baseline ANN. Different shading denotes the specific loss function used during training. Gray horizontal lines denote the individual values.

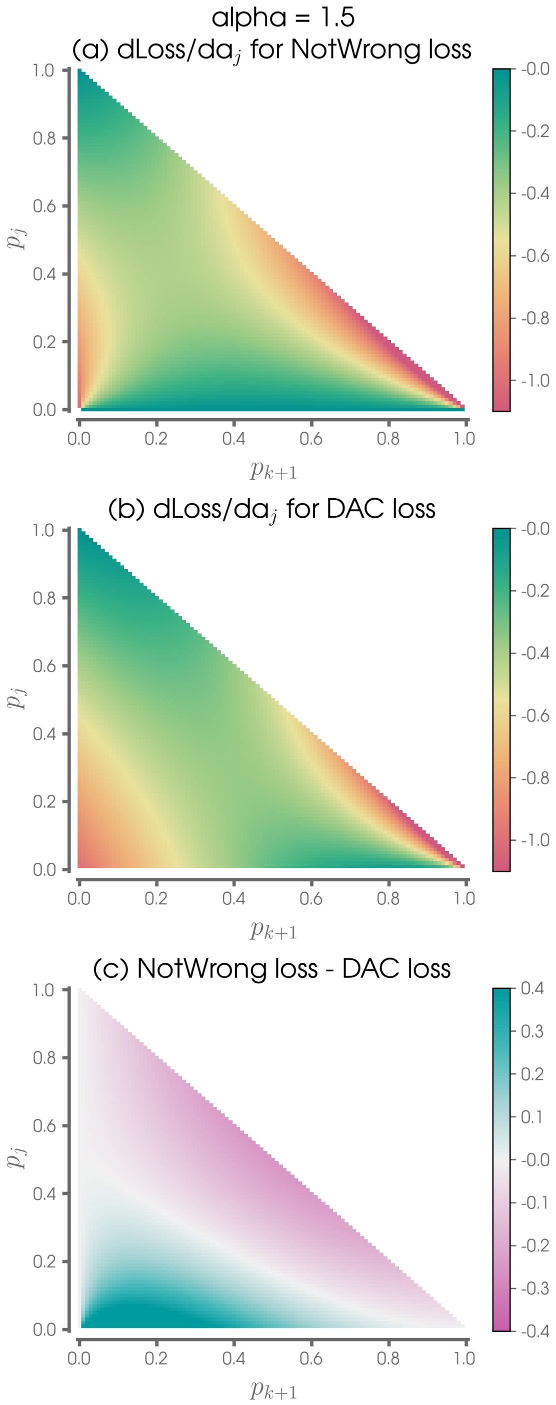


**Figure S3.** (a) Derivative of the NotWrong loss with respect to $a_j$ as a function of $p_j$ and $p_{k+1}$ for $\alpha = 1.5$. (b) As in (a) but for the DAC loss. (c) The difference, where negative values (pink colors) imply that the derivative of the NotWrong loss is more negative than the derivative of the DAC loss.
